# Supplementary material for: The Role of Teacher Calibration in Knowledge Distillation
Source: arXiv:2508.20224 source file (2025-08-27)
Supplement: Supplementary file 1 [file sec_appendix.tex]

% \begin{onecolumn}
% \section*{Appendix}
\section{Property of pretrained teacher models}
\label{subsec:teacher_property}

\begin{table*}[ht]
\centering
\caption{\textbf{Properties of Teacher Models and Student Models used in this paper}: 
This table presents various metrics for teacher models and their corresponding student models' accuracy trained with the standard KD method on the CIFAR-100 dataset.}

\label{tab:tace_sacc}  % \label은 \caption 뒤에 위치해야 함

% \resizebox{\columnwidth}{!}{
\begin{tabular}{ccccccccc}
\toprule
\multicolumn{7}{c}{\textbf{Teacher Properties}} & \multicolumn{2}{c}{\textbf{Student KD Accuracy (\%)}} \\
\cmidrule(r){1-7} \cmidrule(l){8-9}
% \textbf{Model} & \textbf{Accuracy (\%)} & \textbf{ECE (\%)} & $\text{ECE}_{o} (\%)$ & $\text{ECE}_{u} (\%)$ & \textbf{ACE (\%)} & \textbf{Params} & \textbf{WRN-16-2} & \textbf{ShuffleNetV2} \\
\textbf{Model} & \textbf{Accuracy (\%)} & \textbf{ECE (\%)} & \textbf{ECE\(_{o}\) (\%)} & \textbf{ECE\(_{u}\) (\%)} & \textbf{ACE (\%)} & \textbf{Params} & \textbf{WRN-16-2} & \textbf{ShuffleNetV2} \\
\midrule
VGG19      & 74.10 & 16.4723 & 16.4723 & 0.0000 & 0.1336 & 20.1M & 74.42 & 74.17 \\
VGG13      & 74.48 & 8.4570  & 8.3338  & 0.1232 & 0.1048 & 9.5M  & 74.99 & 75.40  \\
VGG16      & 74.66 & 12.8963 & 12.8946 & 0.0017 & 0.1194 & 14.8M & 74.67 & 74.98 \\
ResNet110  & 75.22 & 13.0475 & 13.0475 & 0.0000 & 0.1007 & 1.7M  & 75.48 & 77.04 \\
WRN-28-2   & 75.53 & 7.1268  & 7.1268  & 0.0000 & 0.0924 & 1.5M  & 75.71 & 76.72 \\
WRN-16-3   & 75.98 & 8.7114  & 8.6809  & 0.0305 & 0.0899 & 1.6M  & 76.07 & 77.01 \\
WRN-40-2   & 76.55 & 11.2194 & 11.2003 & 0.0191 & 0.1000 & 2.3M  & 75.51 & 76.11 \\
ResNet18   & 77.43 & 6.9784  & 6.8159  & 0.1625 & 0.0938 & 11.2M & 75.75 & 76.48 \\
WRN-16-4   & 77.69 & 7.5518  & 7.5394  & 0.0124 & 0.0833 & 2.8M  & 76.25 & 76.80  \\
ResNet34   & 78.41 & 9.5015  & 9.4911  & 0.0104 & 0.0902 & 21.3M & 76.03 & 76.62 \\
GoogLeNet  & 78.46 & 6.7732  & 6.7621  & 0.0111 & 0.0762 & 6.4M  & 76.29 & 76.55 \\
WRN-40-4   & 78.51 & 10.3410 & 10.3410 & 0.0000 & 0.0914 & 9.0M  & 75.76 & 76.26 \\
WRN-28-4   & 78.56 & 8.2353  & 8.2353  & 0.0000 & 0.0905 & 5.9M  & 75.59 & 76.90  \\
ResNet32x4 & 78.70 & 9.3010  & 9.2661  & 0.0349 & 0.0840 & 7.4M  & 76.16 & 76.55 \\
WRN-16-6   & 78.79 & 6.3329  & 6.3271  & 0.0058 & 0.0836 & 6.2M  & 76.36 & 77.53 \\
WRN-16-8   & 79.37 & 5.6263  & 5.5865  & 0.0398 & 0.0794 & 11.0M & 76.34 & 76.99 \\
ResNet50   & 79.71 & 7.6640  & 7.6640  & 0.0000 & 0.0790 & 23.7M & 76.12 & 76.91 \\
\bottomrule
\end{tabular}
% }
\end{table*}

Table~\ref{tab:tace_sacc} provides detailed properties of the teacher models that were used in Figure~\ref{fig:ace_sacc} in Section~\ref{subsec:criterion_ace} to demonstrate the correlation between teacher ACE and student accuracy.

Our empirical evaluation across various models in Table~\ref{tab:tace_sacc} confirms that teacher's calibration errors primarily arise from overconfident predictions when models are trained using standard procedures, which justifies our approach to reducing the overconfident calibration error.

\section{Future Work}
% \textbf{Limitations.}
% While this paper empirically demonstrates the significant role of overconfident calibration error in KD, it is important to note that our study is limited in scope to logit distillation methods. Feature distillation is also an important technique widely employed in deep learning applications. We have not explored the impact of calibration error on feature distillation methods, thereby indicating a need for further research in this area.

% \textbf{Future Work.}
The advancement of calibration methods holds considerable promise for their application in knowledge distillation. There are numerous opportunities for integrating more sophisticated calibration techniques into KD pipelines. Future work could involve evaluating the effectiveness of different calibration methods in the KD setting, potentially leading to more robust and accurate student models. Another avenue for research could be to understand the interplay between calibration and other aspects of KD, such as data augmentation, model complexity, and training dynamics. This could yield insights into developing an integrated framework for KD that accounts for both performance and calibration.

% \input{Tables/student_property}

% Table~\ref{tab:student_property} demonstrates the impact of using a teacher with reduced calibration error on the calibration error of the student model. When set to \( T = 1.5 \), we observe a significant reduction in the teacher's overconfident calibration error. Consequently, the student's accuracy improves, accompanied by decreases in both the ECE and the overconfident ECE, as well as the ACE. Notably, in the case of the ResNet32x4-ShuffleNetV1 pair, although the teacher's ACE increases due to an increase in underconfident error, the student's ACE is actually reduced. This suggests that a slightly underconfident teacher, when combined with highly overconfident true labels, enables the student to learn the actual probabilities more effectively. These experimental results validate that our approach not only enhances the accuracy of the student model but also produces a student that is better calibrated. This implies that our approach can yield more reliable models, particularly beneficial when applied in real-world applications.

\section{Societal Impacts}
In this work, we focused on reducing computational resource usage of deep learning models using Knowledge Distillation, whose purpose is to reduce the computational burden of the model while maintaining performance.
We focused on identifying the characteristics of teachers that create effective KD. As a result, we discovered a high correlation between calibration error and KD performance, demonstrating that this can make KD more efficient.
The method proposed in this paper can be applied to various KD methods without any computational overhead and shows robust performance improvement.
These findings can serve as a foundation for future KD research contributing to the reduction of computation and energy use in deploying deep learning models.

% \section{Societal Impacts}
% This work aims to reduce the computational burden of deep learning models through Knowledge Distillation (KD) while maintaining performance. We identify a strong correlation between calibration error and KD effectiveness, suggesting calibration as a key factor in efficient KD.

% Unlike existing KD methods that introduce auxiliary networks or additional losses, increasing computational costs, our approach enhances various KD techniques without extra overhead. These findings contribute to developing energy-efficient deep learning models for real-world deployment.
